# Supplementary material for: Reverse KL-Divergence Training of Prior Networks: Improved Uncertainty and Adversarial Robustness
Source: arXiv:1905.13472 source file (2019-12-02)
Supplement: Supplementary file 1 [file appendix_d.tex]

The current appendix presents out-of-distribution detection results for models trained on the SVHN and CIFAR-100 dataset. On the SVHN datasets Prior Networks were trained using both the forward and reverse KL-divergence losses. The results in table~\ref{tab:svhnOODD} show that both approaches achieve the same performance and outperform ensembles. Here, Prior Networks with forward KL-divergence yield good results because SVHN is a much simpler dataset than CIFAR-10.

\begin{table}[htbp!]
\caption{SVHN out-of-domain detection results in terms of mean \% AUROC $\pm 2\sigma$ across 5 models. Only a single set of results is obtained using explicit ensemble ENSM.}\label{tab:svhnOODD}
\centerline{
\begin{tabular}{ll||cc|ccc}
\toprule
\multirow{2}{*}{OOD Data} & \multirow{2}{*}{Model} & \multicolumn{2}{c|}{Total Uncertainty } &\multicolumn{3}{c}{Knowledge Uncertainty } \\
 & &  Conf. & Ent. & M.I. & EPKL & D.Ent. \\
\midrule
\multirow{3}{*}{CIFAR100} 
& ENSM  & 97.1 \scriptsize{$\pm$ {\tt NA}}& 97.6 \scriptsize{$\pm$ {\tt NA}} & 97.7 \scriptsize{$\pm$ {\tt NA}} & 97.6 \scriptsize{$\pm$ {\tt NA}}& -  \\
& PN-KL  & 99.7 \scriptsize{$\pm 0.1$} & 99.7 \scriptsize{$\pm 0.1$} & 99.7 \scriptsize{$\pm 0.1$} & 89.2 \scriptsize{$\pm 1.0$} & 99.6 \scriptsize{$\pm 0.2$} \\
& PN-RKL & 99.7 \scriptsize{$\pm 0.1$} & \textbf{99.8} \scriptsize{$\pm 0.1$} & \textbf{99.8} \scriptsize{$\pm 0.1$} & \textbf{99.8} \scriptsize{$\pm 0.1$} & \textbf{99.8} \scriptsize{$\pm 0.1$} \\
\midrule
\multirow{3}{*}{LSUN} 
& ENSM & 97.7 \scriptsize{$\pm$ {\tt NA}} & 98.1 \scriptsize{$\pm$ {\tt NA}} & 98.5 \scriptsize{$\pm$ {\tt NA}} & 98.7 \scriptsize{$\pm$ {\tt NA}} & -   \\
& PN-KL  & 100.0 \scriptsize{$\pm 0.0$} & 100.0 \scriptsize{$\pm 0.0$} & 100.0 \scriptsize{$\pm 0.0$} & 88.8 \scriptsize{$\pm 1.1$} & 100.0 \scriptsize{$\pm 0.0$} \\
& PN-RKL & \textbf{100.0} \scriptsize{$\pm 0.0$} & \textbf{100.0} \scriptsize{$\pm 0.0$} & \textbf{100.0} \scriptsize{$\pm 0.0$} & \textbf{100.0} \scriptsize{$\pm 0.0$} & \textbf{100.0} \scriptsize{$\pm 0.0$} \\
\midrule
\multirow{3}{*}{TIM} 
& ENSM & 97.7 \scriptsize{$\pm$ {\tt NA}} & 98.1 \scriptsize{$\pm$ {\tt NA}} & 98.4 \scriptsize{$\pm$ {\tt NA}} & 98.5 \scriptsize{$\pm$ {\tt NA}} & -   \\
& PN-KL  & 100.0 \scriptsize{$\pm 0.0$} & 100.0 \scriptsize{$\pm 0.0$} & 100.0 \scriptsize{$\pm 0.0$} & 88.9 \scriptsize{$\pm 1.1$} & 100.0 \scriptsize{$\pm 0.1$} \\
& PN-RKL & \textbf{100.0} \scriptsize{$\pm 0.0$} & \textbf{100.0} \scriptsize{$\pm 0.0$} & \textbf{100.0} \scriptsize{$\pm 0.0$} & \textbf{100.0} \scriptsize{$\pm 0.0$} & \textbf{100.0} \scriptsize{$\pm 0.0$} \\
\bottomrule
\end{tabular}}
\end{table}

Table~\ref{tab:c100OODD} presents the results of out-of-distribution input detection using Prior Networks trained on the CIFAR-100 data using the reverse KL-divergence loss. In this case, the out-of-distribution training data is the TinyImageNet dataset. 

\begin{table}[htbp!]
\caption{CIFAR-100 out-of-domain detection results in terms of mean \% AUROC $\pm 2\sigma$ across 5 models. In-domain data is CIFAR-100 test set, OOD data is LSUN/SVHN/CIFAR-10 test sets.}\label{tab:c100OODD}
\centerline{
\begin{tabular}{ll||cc|ccc}
\toprule
\multirow{2}{*}{OOD Data} & \multirow{2}{*}{Model} & \multicolumn{2}{c|}{Total Uncertainty } &\multicolumn{3}{c}{Knowledge Uncertainty } \\
 & &  Conf. & Ent. & M.I. & EPKL & D.Ent. \\
\midrule
\multirow{2}{*}{CIFAR10} 
& ENSM   & 75.6 \scriptsize{$\pm$ {\tt NA}} &  \textbf{76.5} \scriptsize{$\pm$ {\tt NA}} &  \textbf{76.5} \scriptsize{$\pm$ {\tt NA}} &  75.6 \scriptsize{$\pm$ {\tt NA}} & - \\
& PN-KL  & 67.6 \scriptsize{$\pm 0.4$} & 67.3 \scriptsize{$\pm 0.5$} & 57.8 \scriptsize{$\pm 0.2$} & 57.0 \scriptsize{$\pm 0.2$} & 62.6 \scriptsize{$\pm 0.6$} \\
\midrule
\multirow{2}{*}{LSUN} 
& ENSM   & 79.4 \scriptsize{$\pm$ {\tt NA}} &  81.6 \scriptsize{$\pm$ {\tt NA}} &  85.6 \scriptsize{$\pm$ {\tt NA}} &  85.2 \scriptsize{$\pm$ {\tt NA}} & - \\
& PN-RKL & \textbf{100.0} \scriptsize{$\pm 0.0$}& \textbf{100.0} \scriptsize{$\pm 0.0$}  &  \textbf{100.0} \scriptsize{$\pm 0.0$} &  \textbf{100.0} \scriptsize{$\pm 0.0$} & \textbf{100.0} \scriptsize{$\pm 0.0$} \\
\midrule
\multirow{2}{*}{SVHN} 
& ENSM    & 72.3 \scriptsize{$\pm$ {\tt NA}} & 75.6 \scriptsize{$\pm$ {\tt NA}} & 78.9 \scriptsize{$\pm$ {\tt NA}} & 78.7 \scriptsize{$\pm$ {\tt NA}} & - \\
& PN-RKL  & 82.7 \scriptsize{$\pm 0.2$} & 84.7 \scriptsize{$\pm 0.4$} & 84.8 \scriptsize{$\pm 0.4$} & 84.6 \scriptsize{$\pm 0.4$} & \textbf{85.7} \scriptsize{$\pm 0.1$} \\
\bottomrule
\end{tabular}}
\end{table}
